# Supplementary material for: BoSy: An Experimentation Framework for Bounded Synthesis
Source: arXiv:1803.09566 source file (2018-03-26)
Supplement: Supplementary file 1 [file appendix.tex]

\section{Examples}

\begin{figure}
\begin{verbatim}
{
    "semantics": "mealy",
    "inputs":  ["r_0", "r_1"],
    "outputs": ["g_0", "g_1"],
    "assumptions": [],
    "guarantees": [
        "G ((!g_0) || (!g_1))",
        "G (r_0 -> (F g_0))",
        "G (r_1 -> (F g_1))"
    ]
}
\end{verbatim}
  \caption{Example JSON input file}
  \label{fig:json_input}
\end{figure}

\begin{figure}
  \centering
  \begin{SubFloat}{\label{fig:aiger_solution}AIGER encoding}
    \begin{minipage}[b]{0.25\linewidth}%  a minipage to control the width...
\begin{verbatim}
aag 3 2 1 2 0
2
4
6 7
6
7
i0 r_0
i1 r_1
l0 s0
o0 g_0
o1 g_1
\end{verbatim}
    \end{minipage}
  \end{SubFloat}%
  \begin{SubFloat}{\label{fig:smv_solution}SMV encoding}
    \begin{minipage}[b]{0.44\linewidth}%  a minipage to control the width...
\begin{verbatim}
MODULE main
  VAR
    state: {s0, s1};
    r_0 : boolean;
    r_1 : boolean;
  ASSIGN
    init(state) := s0;
    next(state) := case
      state = s0 & TRUE : s1;
      state = s1 & TRUE : s0;
    esac;
  DEFINE
    g_0 := (state = s1 & TRUE);
    g_1 := (state = s0 & TRUE);
\end{verbatim}
    \end{minipage}
  \end{SubFloat}%
  \begin{SubFloat}{\label{fig:dot_solution}graph representation}
    \begin{minipage}[b]{0.25\linewidth}%  a minipage to control the width...
      \includegraphics[width=\linewidth]{./dot_solution}
    \end{minipage}
  \end{SubFloat}

  \caption{Different encodings of the controller synthesized by $\bosy$ given the specification in Fig.~\ref{fig:json_input}.}
  \label{fig:synthesized}
\end{figure}
